# Supplementary material for: Domain Randomization is Sample Efficient for Linear Quadratic Control
Source: arXiv:2502.12310 source file (2025-02-17)
Supplement: Supplementary file 1 [file CE_appendix_unused.tex]

\section{Upper Bound for the CE Controller Proofs}
The Taylor's expansion of $C(K(\hat\theta), \theta^\star)$ evaluated at $\theta^\star$ gives us
\begin{align*}
    &C(K(\hat{\theta}), \theta^\star)) - C(K(\theta^\star), \theta^\star) \\ 
    &= \frac{1}{2}
    [\hat\theta - \theta^\star]^T\left(\left.\frac{\partial K(\theta)}{\partial \theta}\right|_{\theta = \theta^\star}\right)^T
    \left.\frac{\partial^2 C(K(\theta), \theta^\star)}{\partial K(\theta)^2}\right|_{K(\theta) = K(\theta^\star)}
    \left.\frac{\partial K(\theta)}{\partial \theta}\right|_{\theta = \theta^\star}
    [\hat{\theta} - \theta^\star] \\
    &+ \frac{1}{6}
    \left.\frac{\partial^3 C(K(\theta), \theta^\star)}{\partial K(\theta)^3}\right|_{K(\theta) = K(\theta')}
    \left[\left.\frac{\partial K(\theta)}{\partial \theta}\right|_{\theta = \theta'}
    (\hat{\theta} - \theta^\star), 
    \left.\frac{\partial K(\theta)}{\partial \theta}\right|_{\theta = \theta'}(\hat{\theta} - \theta^\star), 
    \left.\frac{\partial K(\theta)}{\partial \theta}\right|_{\theta = \theta'}(\hat{\theta} - \theta^\star)\right] \\
    &+ \frac{1}{2}
    \left.\frac{\partial^2 C(K(\theta), \theta^\star)}{\partial K(\theta)^2}\right|_{K(\theta) = K(\theta')}
    \left[\left.\frac{\partial^2 K(\theta)}{\partial \theta^2}\right|_{\theta = \theta'}
    [\hat{\theta} - \theta^\star,\hat{\theta} - \theta^\star] ,
    \left.\frac{\partial K(\theta)}{\partial \theta,}\right|_{\theta = \theta'}(\hat{\theta} - \theta^\star)\right] 
\end{align*}
where $\theta' = \theta^\star + t(\hat\theta - \theta^\star)$ for $t\in[0,1]$, and we used $\frac{\partial C(K(\theta^\star), \theta^\star)}{\partial K(\theta)}= 0$ since $K_{CE}(\theta^\star) = \argmin_KC(K, \theta^\star)$.

From (\ref{eq:d2C/dK2 bound}), (\ref{eq:d3C/dK3 bound}), (\ref{eq:PK bound}),(\ref{eq:dk/dtheta bound}), (\ref{eq:dk/dtheta bound}), (\ref{eq:d2k/dtheta2 bound}), (\ref{eq:P(A',B') bound}), the upper bound on the CE controller is given as
\begin{align*}
    &C(K(\hat{\theta}), \theta^\star)) - C(K(\theta^\star), \theta^\star) \\ 
    &\leq \frac{1}{2}
    [\hat\theta - \theta^\star]^T\left(\left.\frac{\partial K(\theta)}{\partial \theta}\right|_{\theta = \theta^\star}\right)^T
    \left.\frac{\partial^2 C(K(\theta), \theta^\star)}{\partial K(\theta)^2}\right|_{K(\theta) = K(\theta^\star)}
    \left.\frac{\partial K(\theta)}{\partial \theta}\right|_{\theta = \theta^\star}
    [\hat{\theta} - \theta^\star] \\
    &+\frac{7^3}{6}\left(\frac{21}{20}\right)^{9/2}\left(\frac{11}{10}\right)^{21/2}(68\|B\|_F^3 + 28\|B\|_F^2 + 6\|B\|_F)\|\Sigma_w\|_F\|P_\star\|^{15}_{op}\|\hat\theta - \theta^\star\|_2^3 \\
    &+1015\left(\frac{21}{20}\right)^3\left(\frac{11}{10}\right)^{11}(10\|B\|_F^2 + 4\|B\|_F + 1)\|\Sigma_w\|_F\|P_\star\|^{14}_{op}\|\hat\theta - \theta^\star\|_2^3
\end{align*}
if $\epsilon_{op}\leq\frac{1}{54}\|P_\star\|_{op}^{-5}$.

From \Cref{thm: identification bound}, we get
\begin{align*}
    &C(K(\hat{\theta}), \theta^\star)) - C(K(\theta^\star), \theta^\star) \\ 
    &\leq \frac{1}{2}\|\hat{\theta} - \theta^\star\|_H + 
    poly(\|B\|_F, \|\Sigma_w\|_F)\|P_\star\|^{15}_{op}\|\hat\theta - \theta^\star\|^3_2
    \\
    &\leq 2 \frac{\trace\paren{H \mathsf{FI}(\theta^\star)^{-1}}}{N} + 4 \frac{\norm{H \mathsf{FI}(\theta^\star)^{-1}}}{N} \log\frac{2}{\delta} 
    + \frac{poly(\|B\|_F, \|\Sigma_W\|_F, \mathsf{FI}(\theta^\star), \delta)\|P_\star\|^{15}_{op}}{N^{3/2}}
\end{align*}
as long as $N \geq N_{\mathsf{ID}}$. 

\subsection{Norm bound on $\frac{\partial C}{\partial K}, \frac{\partial^2 C}{\partial K^2}, \frac{\partial^3 C}{\partial K^3}$}
Consider the perturbation of any $K$ along any matrix $\Delta$:
\begin{align}
    K(t) = K + t\Delta, ~ t \in \R \label{eq:K(t)}, ~ \|\Delta\|_F\leq1.
\end{align}
Let us adopt shorthand $(\cdot) \triangleq \frac{d}{dt}(\cdot)$. Then the norm bound on $\frac{\partial C}{\partial K}$ would be
\begin{align*}
    \left\|\frac{\partial C}{\partial K}\right\|_{op} &= \sup_{\|\Delta\|_F\leq1}\left|\frac{d}{dt}C(K+t\Delta, \theta^\star)|_{t=0}\right| = \sup_{\|\Delta\|_F\leq1} Tr(P'_K(0)\Sigma_w) \leq \sup_{\|\Delta\|_F\leq1}\|P_K'(0)\|_F\|\Sigma_w\|_F
\end{align*}
where $P_K(t)$ is the solution to the following Lyapunov equation:
\begin{align*}
    P_K(t) &= (A + BK(t))^TP_K(t)(A + BK(t)) + Q + K(t)^TRK(t) \\
    &= \dlyap(A+BK(t), Q + K(t)^TRK(t)).
\end{align*}
By taking the derivative, $P_K'(t)$ is given as 
\begin{align*}
    P_K'(t) &= \dlyap(A+BK(t), Q_1(t)) \\
    Q_1(t) &= \sym((A+BK(t))^TP_K(t)B\Delta) + \sym(K(t)^TR\Delta)
\end{align*}
where we used the notation $\sym(X) = X + X^T$. 
Then the norm bound on $P'_K(t)$ is given as
\begin{align}
    \|P_K'(t)\|_o &= \|\dlyap(A + BK(t), Q_1)\|_o \nonumber\\
    &\leq \|\dlyap(A+BK(t),I)\|_{op}\|Q_1\|_{o} \nonumber\\
    &\leq \|P_K(t)\|_{op}\|Q_1\|_o \nonumber\\
    &\leq 2\|P_K(t)\|^{5/2}_{op}\|B\|_o + \|P_K(t)\|^{3/2}_{op} \nonumber \\
    &\leq (2\|B\|_o+1)\|P_K(t)\|^{5/2}_{op}    \label{eq:Pk' bound} 
\end{align}
where the norm bound on $Q_1$ is given as 
\begin{align*}
    \|Q_1\|_{o} &\leq 2\|A+BK(t)\|_{o}\|P_K(t)\|_{op}\|B\Delta\|_{o} + 2\|K(t)\|_{op}\|R\Delta\|_o \\
    &\leq 2\|P_K(t)\|^{3/2}_{op}\|B\|_o + \|P_K(t)\|^{1/2}_{op} \hspace{5mm} \because R = I, \|\Delta\|_o\leq1
\end{align*}
Thus 
\begin{align}
    \left\|\left.\frac{\partial C(K(\theta), \theta^\star)}{\partial K}\right|_{K(\theta) = K(\theta')}\right\|_{op} 
    &\leq (2\|B\|_F+1)\|P_{K(\theta')}(0)\|^{5/2}_{op} \|\Sigma_w\|_F \label{eq:dC/dK bound}
\end{align}
Also the second derivative is given as
\begin{align*}
    P''_K(t) &= \dlyap(A+BK(t), Q_2) \\
    Q_2 &= 2\{sym((A+BK(t))^TP_K'(t)B\Delta) + (B\Delta)^TP_K(t)B\Delta + \Delta^TR\Delta\}
\end{align*}
Then the norm bound would be
\begin{align*}
    \|P_K''(t)\|_o &= \|\dlyap((A+BK(t)), Q_2)\|_o \\
    &\leq \|P_K(t)\|_{op}\|Q_2\|_o \\
    &\leq (10\|B\|_o^2 + 4\|B\| + 1)\|P_K(t)\|^{3}_{op}
\end{align*}
where, from (\ref{eq:Pk' bound}), 
\begin{align*}
    \|Q_2\|_o &\leq 4\|A+BK(t)\|_o\|P_K'(t)\|_{op}\|B\Delta\|_o + 2\|B\Delta\|_o^2\|P_K(t)\|_{op} + \|R^{1/2}\Delta\|^2_o \\
    &\leq 4\|B\|_o(2\|B\|_o+1)\|P_K(t)\|^{3}_{op} + 2\|B\|_o^2\|P_K(t)\|_{op} + 1 \\
    &\leq (10\|B\|_o^2 + 4\|B\| + 1)\|P_K(t)\|^{3}_{op}
\end{align*}
Therefore
\begin{align}
    &\left\|\left.\frac{\partial^2 C(K(\theta),\theta^\star)}{\partial K^2}\right|_{K(\theta) = K(\theta')}\right\|_{op} 
    \leq (10\|B\|_F^2 + 4\|B\|_F + 1)\|P_{K(\theta')}(0)\|^{3}_{op}\|\Sigma_w\|_F \label{eq:d2C/dK2 bound} 
\end{align}

Finally the third derivative is 
\begin{align*}
    P'''_K(t) &= \dlyap(A+BK, Q_3) \\
    Q_3 &= 3sym((A+BK(t))^TP_K''(t)B\Delta) + 4(B\Delta)^TP_K'(t)B\Delta 
\end{align*}
Then the norm bound would be
\begin{align*}
    \|P'''_K(t)\|_o &\leq \|Q_3\|_o\|P_K(t)\|_{op} \\
    &\leq (68\|B\|_o^3 + 28\|B\|_o^2 + 6\|B\|_o)\|P_K(t)\|^{9/2}_{op}
\end{align*}
where 
\begin{align*}
    \|Q_3\|_o &\leq 6\|A+BK(t)\|_o\|P_K''(t)\|_{op}\|B\Delta\|_o + 4\|P_K'(t)\|_{op} \|B\Delta\|_o^2 \\
    &\leq 6\|B\|_o(10\|B\|_o^2 + 4\|B\|_o + 1)\|P_K(t)\|^{7/2}_{op} + 4\|B\|_o^2(2\|B\|_o+1)\|P_K(t)\|^{5/2}_{op} \\
    &\leq (68\|B\|_o^3 + 28\|B\|_o^2 + 6\|B\|_o)\|P_K(t)\|^{7/2}_{op}
\end{align*}
thus 
\begin{align}
    \left\|\left.\frac{\partial^3 C(K(\theta), \theta^\star)}{\partial K^3}\right|_{K(\theta) = K(\theta')}\right\|_{op}\leq (68\|B\|_F^3 + 28\|B\|_F^2 + 6\|B\|_F)\|P_{K(\theta')}(0)\|^{9/2}_{op}\|\Sigma_w\|_F 
    \label{eq:d3C/dK3 bound}
\end{align}

From Theorem 5 in \citep{simchowitz2020naive}, the bound on $\|P_{K(\theta')}(0)\|_{op}$ is given as follows: if $\epsilon_{op}\leq\frac{1}{54}\|P_\star\|_{op}^{-5}$, we get
\begin{align}
    P_{K(\theta')}(0) \preceq \frac{21}{20}P_\star  \label{eq:PK bound}
\end{align}
% Note that this satisfies the necessary condition $\|B(K(\theta') - K(\theta^\star))\|_2 \leq \frac{1}{5}\|P_\star\|_{op}^{-3/2}$.



\subsection{Norm bound on $\frac{\partial K}{\partial \theta}, \frac{\partial^2 K}{\partial \theta^2}$}
Consider the perturbation of A and B, i.e.
\begin{align*}
    (A(t), B(t)) = (A_* + t\Delta_1, B_* + t\Delta_2)
\end{align*}
where $\|\Delta_1\|_F, \|\Delta_2\|_F\leq1, t\in\R$.
As long as $(A(t), B(t))$ is stabilizable, the discrete algebraic ricatti equation has a unique solution and associated optimal cost matrices, controllers, and closed-loop dynamics matrices are defined as
\begin{align*}
    P(t) \triangleq P_{\infty}(A(t), B(t)), ~ K(t) \triangleq K_{\infty}(A(t), B(t)), ~ A_{cl}(t) \triangleq A(t) + B(t)K(t)
\end{align*}
where $P_{\infty}$ is the solution of
\begin{align*}
    \dare([A, B], P) = A^TPA - P - A^TPB(R + B^TPB)^{-1}B^TPA + Q 
\end{align*}
and $K_{\infty} \triangleq argmin_{K}C(K, \theta^*)$ is given by
\begin{align}
    K(t) = -(R + B^TPB)^{-1}B^TPA \label{eq:K_inf}
\end{align}

By taking the derivative of $P(t)$, we get
\begin{align*}
    P'(t) &= \dlyap(A_{cl}(t), Q_4(t)) \\
    Q_4(t) &= \sym(A_{cl}^TP(t)\Delta_{A_{cl}}), ~ \Delta_{A_{cl}} = \Delta_1 + \Delta_2K(t)
\end{align*}
Thus the norm bound on $P'(t)$ is given by
\begin{align*}
    \|P'(t)\|_o &= \|dlyap(A_{cl}(t), Q_4(t)\|_o 
    \\
    &\leq \|dlyap(A_{cl}(t), I)\|_{op}\|Q_4(t)\|_o &\because  B.5
    \\
    &\leq \|P(t)\|_{op}\cdot2(\|A_{cl}(t)\|_{op}\|P(t)\|_{op}\|\Delta_{A_{cl}}\|_o) &\because B.5\\
    &\leq 2\|P(t)\|^2_{op}\|P(t)\|^{1/2}_{op}\cdot2\|P(t)\|_{op}^{1/2}&\because  B.8, C.3\\
    &= 4\|P(t)\|^3_{op}
\end{align*}
where $\|\Delta_{A_{cl}}\|_o \leq \|\Delta_1\|_o + \|\Delta_2\|_o\|K\|_{op}\leq
1 + \|K\|_{op} \leq 2\|P(t)\|_{op}^{1/2}$

Also the derivative of $K(t)$ is
\begin{align*}
    K'(t) = -(R + B^TPB)^{-1}\left(\Delta_2^TPA_{cl} + B^TP\Delta_{A_{cl}} + B^TP'A_{cl}\right)
\end{align*}
Let $R_0 = R + B^TPB$. 
Then the norm bound is given by
\begin{align*}
    \|K'(t)\|_o &\leq \|R_0^{-1}\|_{op}\|\Delta_2\|_{o}\|P\|_{op}\|A_{cl}\|_{op} + \|P\|^{1/2}_{op}\|\Delta_{A_{cl}}\|_{o} + \|P^{-1/2}\|_{op}\|P'\|_{op}\|A_{cl}\|_{op} \\
    &\leq 7\|P(t)\|^{7/2}_{op}
\end{align*}
where we used $\|R_0^{-1}B^TP^{1/2}\|_{op}\leq1 (\because$ C.3).

Then the norm bound of the first derivative is given by
\begin{align}
    \left\|\left.\frac{\partial K(\theta)}{\partial\theta}\right|_{\theta = \theta'}\right\|_{op} \leq 7\|P_{\infty}(A', B')\|_{op}^{7/2} \label{eq:dk/dtheta bound}
\end{align}

Also, $P''(t)$ is calculated as follows
\begin{align*}
    P''(t) &= \dlyap(A_{cl}, Q_5) \\
    Q_5 &= \sym(A_{cl}'P'A_{cl}) + \sym(A_{cl}'P\Delta_{A_{cl}}) + \sym(A_{cl}^TP\Delta_{A_{cl}}') + \sym(A_{cl}^TP'\Delta_{A_{cl}}')
\end{align*}
Therefore we get
\begin{align*}
    \|P''(t)\|_o &\leq \|P\|_{op}\|Q_5\|_o \\
    &\leq 2\|P\|_{op}(\|A_{cl}'\|\|P'\|\|A_{cl}\| + \|A_{cl}'\|\|P\|\|\Delta_{A_{cl}}\| + \|A_{cl}\|\|P\|\|\Delta_{A_{cl}}'\| + \|A_{cl}\|\|P'\|\|\Delta_{A_{cl}}'\|) \\
    &\leq 2\|P\|_{op}(36\|P\|^7 + 18\|P\|^5 + 7\|P\|^5 + 28\|P\|^5 &\because C.4 \\
    &\leq 178\|P(t)\|^7
\end{align*}

For K'', let $Q_6 = \Delta_B^TPA_{cl} + B^TP\Delta_{A_{cl}} + B^TP'A_{cl}$. Then 
\begin{align*}
    K'' = -R_0^{-1}Q_6' - R_0^{-1}R_0'K'
\end{align*}
Since $Q_6'$ is given as
\begin{align*}
    Q_6' &= \Delta_B^TP'A_{cl} + \Delta_B^TPA_{cl}' + \Delta_B^TP\Delta_{A_{cl}} + B^TP'\Delta_{A_{cl}} +B^TP\Delta_{A_{cl}}' + \Delta_B^TP'A_{cl} + B^TP''A_{cl} + B^TP'A_{cl}' \\
    &=\Delta_B^T(2P'A_{cl} + PA_{cl}' + P\Delta_{A_{cl}}) + B^T(P\Delta_{A_{cl}}' + P'A_{cl}' + P'\Delta_{A_{cl}} + P''A_{cl})
\end{align*}
we get the following norm bound 
\begin{align*}
    \|R_0^{-1}Q_6'\|_o &\leq \|R_0^{-1}\|(2\|P'\|\|P\|^{1/2} + 9\|P\|\|P\|^{7/2} + 2\|P\|\|P\|^{1/2}) \\
    &\hspace{5mm} + \|R_0^{-1}B\|(7\|P\|\|P\|^{7/2}+ 9\|P'\|\|P\|^{7/2} + 2\|P'\|\|P\|^{1/2} + \|P''\|\|P\|^{1/2}) \\
    &\leq 8\|P\|^{7/2} + 9\|P\|^4 + 2\|P\|^{3/2} + 7\|P\|^8 + 36\|P\|^{13/2} + 8\|P\|^{7/2} + 178\|P\|^{15/2} \\
    &\leq 248\|P\|^{15/2}
\end{align*}
For the second term, we get
\begin{align*}
    \|R_0^{-1}R_0'K'\|_o &\leq \|R_0^{-1}(B'^TPB + B^TP'B + B^TPB')K'\| \\
    &\leq (\|R_0^{-1}\|\|P\| + \|R_0^{-1}B\|\|P'\|)\|BK'\| + \|R_0^{-1}B\|\|P\|\|K'\| \\
    &\leq (\|P\| + 4\|P\|)\|BK'\| + \|P\|\|P\|^{7/2}\\
    &\leq 35\|P\|^{9/2} + 7\|P\|^{9/2} \\
    &\leq 42\|P\|^{9/2}
\end{align*}
Thus the norm bound on K'' is
\begin{align*}
    \|K''(t)\|_o &\leq 290\|P(t)\|^{15/2}_{op}
\end{align*}
Thus
\begin{align}
    \left\|\left.\frac{\partial^2 K(\theta)}{\partial\theta^2}\right|_{\theta=\theta'}\right\|_{op}
    &\leq 290\|P_{\infty}(A', B')\|^{15/2}_{op}\label{eq:d2k/dtheta2 bound}
\end{align}

Again from Theorem 5 in \citep{simchowitz2020naive}, the norm bound on $P_{\infty}(A', B')$ is given as follows: if $\epsilon_{op}\leq\frac{1}{54}\|P_\star\|_{op}^{-5}$, we get
\begin{align}
    \|P_{\infty}(A', B')\|_{op} \leq \frac{11}{10}\|P_\star\|_{op} \label{eq:P(A',B') bound}
\end{align}
