# Supplementary material for: Domain Randomization is Sample Efficient for Linear Quadratic Control
Source: arXiv:2502.12310 source file (2025-02-17)
Supplement: Supplementary file 2 [file RC_appendix_unused.tex]

\section{Proof of Robust Control Upper Bound (Unused)}
\begin{enumerate}
\item Let $G = \{\theta : (\theta - \hat\theta)^T\mathsf{\hat{FI}}(\hat\theta)(\theta-\hat\theta)\leq8(d_x+\log\frac{1}{\delta})\}$ be the confidence region around $\hat\theta$. From \cref{thm: identification bound}, $\theta^\star\in G$ with probability at least $1-\delta$. 
\item Let the robust controller be 
\begin{align*}
    {K}_{RC}(G) = \argmin_{K}\sup_{\theta\in G}(C(K, {\theta}) - C(K(\theta), {\theta})).
\end{align*}
\item When $\theta^\star\in G$, the suboptimality gap is given by
\begin{align*}
    C(K_{RC}(G), \theta^\star) - C(K(\theta^\star), \theta^\star) 
    &\leq \sup_GC(K_{RC}(G), \theta) - C(K(\theta), \theta) \\
    &= \inf_K\sup_GC(K, \theta) - C(K(\theta), \theta)
\end{align*}
Now, assuming $\Sigma_w = I$, we get 
\begin{align*}
    &C(K,\theta) - C(K(\theta), \theta) \\
    &= \trace(P_K) - \trace (P_{K(\theta)}) \\
    &= \trace (\dlyap (A+BK, (K-K(\theta)^T\Psi(\theta)(K-K(\theta)))) \\
    &= \trace ((K-K(\theta))\Sigma_X^K(\theta)(K-K(\theta))^T\Psi(\theta)) \\
    &= \trace ((K-K(\theta))\Sigma_X^{K(\theta)}(\theta)(K-K(\theta))^T\Psi(\theta) + (K-K(\theta))(\Sigma_X^K(\theta) - \Sigma_X^{K(\theta)}(\theta))(K-K(\theta))^T\Psi(\theta))
\end{align*}
where $\Psi(\theta) = R + B^TP(\theta)B, \Sigma_X^K(\theta) = \dlyap((A+BK)^T, I)$ and used
\begin{align*}
    \trace(\dlyap(X,Y)) &= \trace\left(\sum_{t=0}^{\infty}(X^t)^TYX^t\right) \\
    &= \trace \left(Y\sum_{t=0}^{\infty}(X^t)^TX^t\right)\\
    &= \trace (Y\dlyap(X^T, I))
\end{align*}

\item For any $K_1, K_2$, 
\begin{align*}
    \Sigma_X^{K_1} - \Sigma_X^{K_2} &= \dlyap((A+BK_1)^T, I) - \dlyap((A+BK_2)^T, I) \\
    &= (A+BK_1)\Sigma_X^{K_1}(A+BK_1)^T - (A+BK_2)\Sigma_X^{K_2}(A+BK_2)^T \\
    &= (A+BK_2+B(K_1-K_2))\Sigma_X^{K_1}(A+BK_2+B(K_1-K_2))^T \\
    & \hspace{5mm}- (A+BK_2)\Sigma_X^{K_2}(A+BK_2)^T \\
    &= (A+BK_2)(\Sigma_X^{K_1}-\Sigma_X^{K_2})(A+BK_2)^T + B(K_1-K_2)\Sigma_X^{K_1}(K_1-K_2)^TB^T\\
    &\hspace{5mm}+ (A+BK_2)\Sigma_X^{K_1}(K_1-K_2)^TB^T + B(K_1-K_2)\Sigma_X^{K_1}(A+BK_2)^T \\
    &= \dlyap(A+BK_2, B(K_1-K_2)\Sigma_X^{K_1}(K_1-K_2)^TB^T \\
    &\hspace{5mm}+ \sym((A+BK_2)\Sigma_X^{K_1}(K_1-K_2)^TB^T))
\end{align*}
Thus for $K, K(\theta)$, we get
\begin{align*}
    \|\Sigma_X^{K} - \Sigma_X^{K_\theta}\| 
    &\leq \|\dlyap(A+BK(\theta), I)\|(\|\Sigma_X^{K}\|\|B\|^2\|K-K(\theta)\|^2 \\
    &\hspace{5mm}+ 2\|A+BK(\theta)\|\|\Sigma_X^{K}\|\|K-K(\theta)\|\|B\|) \\
    &\leq \|\|\Sigma_X^{K(\theta)}\|\|\|\Sigma_X^{K}\|\|B\|\|K-K(\theta)\|(\|B\|\|K-K(\theta)\| + 2\|A+BK(\theta)\|)
\end{align*}

\item The suboptimality gap would be
\begin{align*}
    &C(K_{RC}(G), \theta^\star) - C(K(\theta^\star), \theta^\star) \\
    &\leq \inf_K\sup_G \trace ((K-K(\theta))\Sigma_X^{K(\theta)}(\theta)(K-K(\theta))^T\Psi(\theta)) \\
    &\hspace{5mm}+ \|\Sigma_X^{K(\theta)}(\theta)\|\|\Sigma_X^{K}(\theta)\|\|B\|\|K-K(\theta)\|^3\|\Psi(\theta)\|(\|B\|\|K-K(\theta)\| + 2\|A+BK(\theta)\|)\Tesshu{\times du?} \\
    &\triangleq UB(K, \Sigma_X^K(\theta), \theta)
\end{align*}

\item Restricting the class over $K$ to CE policies yields
\begin{align*}
    C(K_{RC}(G), \theta^\star) - C(K(\theta^\star), \theta^\star) &\leq \inf_{\tilde\theta}\sup_{\theta\in G} UB(K(\tilde\theta), \Sigma_X^{K(\tilde\theta)}(\theta), \theta) \\
    &\leq \inf_{\tilde\theta_1}\sup_{\tilde\theta_2, \theta\in G}UB(K(\tilde\theta_2), \Sigma_X^{K(\tilde\theta_1)}(\theta), \theta)
\end{align*}

Also, let us introduce the stabilizablity condition
\begin{definition}
    Let $\tau, r\in\R_{++}$. An instance $(A, B, \theta^\star, Q, R)$ is $(\tau,r)$-robustly LQR stabilizable if for any $G\subseteq\mathcal{B}(\theta^{\star}, r)$, there exists $\tilde\theta\in G$ such that, for any $\theta\in G$, 
    \begin{align*}
        \|\Sigma_X^{K(\tilde\theta)}\|\leq\tau
    \end{align*}
\end{definition}

\item Fix any $r$, and let $\tau$ be the smallest number such that $(A, B, \theta^\star, Q, R)$ is $(\tau, r)$-robustly stabilizable. Also let $N$ be sufficiently large that $G\subseteq\mathcal{B}(\theta^{\star}, r)$ with high probability. Then it holds by definition that $ \|\Sigma_X^{K(\tilde\theta)}\|\leq\tau$. Thus we get
\begin{align*}
    &C(K_{RC}(G), \theta^\star) - C(K(\theta^\star), \theta^\star) \\
    &\leq \inf_{\tilde\theta_1}\sup_{\tilde\theta_2, \theta\in G} \trace ((K(\tilde\theta_2)-K(\theta))\Sigma_X^{K(\theta)}(\theta)(K(\tilde\theta_2)-K(\theta))^T\Psi(\theta)) \\
    &\hspace{5mm}+ \tau\|\Sigma_X^{K(\theta)}(\theta)\|^{1/2}\|B\|\|K(\tilde\theta_2)-K(\theta)\|^3\|\Psi(\theta)\|(\|B\|\|K(\tilde\theta_2)-K(\theta)\| + 2\|A+BK(\theta)\|)
\end{align*}

For the first term, we get
\begin{align*}
    &\trace ((K(\tilde\theta_2)-K(\theta))\Sigma_X^{K(\theta)}(\theta)(K(\tilde\theta_2)-K(\theta))^T\Psi(\theta)) \\
    &= \VEC(K(\tilde\theta_2) - K(\theta))(\Psi(\theta)\kron\Sigma_X^{K(\theta)})\VEC(K(\tilde\theta_2)-K(\theta)) \\
    &= \|\tilde\theta_2-\theta\|_{K'(\theta)^T(\Psi(\theta)\kron\Sigma_X^{K(\theta)})K'(\theta)} + h.o.t ~\Tesshu{\text{need to explicitly calculate?}}
\end{align*}
where we used the following decomposition from the mean value theorem:
\begin{align*}
    \VEC(K(\tilde\theta_2)-K(\theta)) &= K'(\theta')[\tilde\theta_2 - \theta] \\
    &= K'(\theta)[\tilde\theta_2 - \theta] + \left(K'(\theta') - K'(\theta)\right)[\tilde\theta_2 - \theta]
\end{align*}
where $\theta' = \theta + t(\tilde\theta_2 - \theta)$ and $K'(\theta') \triangleq \left.\frac{\partial K}{\partial \theta}\right|_{\theta = \theta'}$. 
Taking the supremum of $\tilde\theta_2, \theta$ over $G$ yields
\begin{align*}
    \sup_{\tilde\theta_2, \theta\in G}\|\tilde\theta_2 - \theta\|_{H(\theta)} \leq \sup_{\theta\in G}16(d_x + log1/\delta)\|\mathsf{\hat{FI}}(\hat\theta)^{-1}H(\theta)\|
\end{align*}
where $H(\theta) = K'(\theta)^T(\Psi(\theta)\kron\Sigma_X^{K(\theta)})K'(\theta)$. 
\Tesshu{Bound $H(\theta)$}
Let $M(\theta) = (\Psi(\theta)\kron\Sigma_X^{K(\theta)})$. Then
\begin{align*}
    &H(\theta) - H(\theta^\star) \\
    &= K'(\theta)^TM(\theta)K'(\theta) - K'(\theta^\star)^TM(\theta^\star)K'(\theta^\star) \\
    &= K'(\theta^\star)^TM(\theta)K'(\theta) + (K'(\theta) - K'(\theta^\star)^TM(\theta)(K'(\theta) - K'(\theta^\star)) + 2K'(\theta^\star)^TM(\theta)(K'(\theta) - K'(\theta^\star)) \\
    &\hspace{5mm}- K'(\theta^\star)^TM(\theta^\star)K'(\theta^\star) \\
    &\leq K'(\theta^\star)^TM(\theta)K'(\theta) - K'(\theta^\star)^TM(\theta^\star)K'(\theta^\star)
    + \|K''(\theta')\|^2\|\theta-\theta^\star\|^2\|M(\theta)\| \\
    &\hspace{5mm}+ 2\|K'(\theta^\star)\|\|M(\theta)\|\|\|K''(\theta)\|\|\theta-\theta^\star\|\\
    &=  K'(\theta^\star)^T(M(\theta) - M(\theta^\star))K'(\theta^\star) + \|K''(\theta')\|^2\|\theta-\theta^\star\|^2\|M(\theta)\| \\
    &\hspace{5mm}+ 2\|K'(\theta^\star)\|\|M(\theta)\|\|\|K''(\theta)\|\|\theta-\theta^\star\| \\
    &\leq \|K'(\theta^\star)\|^2\|M(\theta) - M(\theta^\star)\| + \|K''(\theta')\|^2\|\theta-\theta^\star\|^2\|M(\theta)\|\\
    &\hspace{5mm}+ 2\|K'(\theta^\star)\|\|M(\theta)\|\|\|K''(\theta)\|\|\theta-\theta^\star\|
\end{align*}


For the second term, from Proposition 4 in \citep{simchowitz2020naive}, if $u\triangleq8\|P_\star\|_{op}^2\epsilon_{op}<1$, $\hat\theta$ is stabilizable and the following bound holds:
\begin{align*}
    \|K(\hat\theta) - K_\star\|_o \leq 7(1-u)^{-7/4}\|P_\star\|_{op}^{7/2}\epsilon_o
\end{align*}
Thus if $G$ is small enough that $\theta^\star\in G$, then
\begin{align*}
    \sup_{\tilde\theta_2,\theta\in G}\|K(\tilde\theta_2) - K(\theta)\|
    &\leq 2\sup_{\theta\in G}\|K(\theta) - K(\theta^\star)\| \Tesshu{\text{does it hold?}} \\
    &\leq 14(1-u)^{-7/4}\|P_\star\|_{op}^{7/2}\epsilon_o
\end{align*}
as long as $\|\theta-\theta^\star\|_{op}\leq\frac{1}{16}\|P_\star\|_{op}^2$

\end{enumerate}
